# Supplementary material for: Improving Faithfulness of Abstractive Summarization by Controlling Confounding Effect of Irrelevant Sentences
Source: arXiv:2212.09726 source file (2024-01-18)
Supplement: Supplementary file 1 [file bart_score.tex]

\section{Automatic Evaluation Metrics}
\label{app:autoevals}
We use ROUGE~\cite{lin-2004-rouge} for automatic evaluation of our model, but as shown in previous works~\cite{cohan-goharian-2016-revisiting, bhandari-etal-2020-evaluating}, it may not correlate well with the human perception of generation quality. Furthermore, we observed that ROUGE in particular falls short of measuring the \textit{multiperspectivity} and \textit{faithfulness} of the generated summary. We address the former issue by introducing a new metric and the latter by modifying BARTScore~\cite{yuan2021bartscore} for our setting. We also report METEOR scores \cite{banerjee2005meteor} for all models since it weighs recall higher than precision and can serve as a proxy for measuring multiperspectivity.
Lastly, we explored using another popular metric BERTScore~\cite{BERTScore} to evaluate our models. We found the BERTScores for our models to be saturated where all models scored in excess of 95 F1-score.

\section{\bartscore{} for answer summarization}
\label{app:bart_score}

\paragraph{Can BARTScore evaluate faithfulness of answer summarization tasks?}
An abstractive model output summary is considered \emph{faithful} to its input if the summary is free from intrinsic and extrinsic hallucinations. In other words, a summary is faithful if it is entailed by the answers. Automatic evaluation of faithfulness or factual correctness of abstractive summaries is still an open problem \citep{surveyevaltextgen}. Earlier works  ~\citet{falke2019ranking,gabriel-etal-2021-go} also show that that out-of-the-box entailment models trained on NLI datasets fail to evaluate factuality of the generated output summaries and do not correlate strongly with the ROUGE scores.
A recent study by \citet{yuan2021bartscore} also shows that the log-likelihood scores of strong generative models like BART (referred to as \bartscore{} in their paper) can correlate well with human generated factuality scores. Specifically, they show that compared to the other metrics, the \bartscore{} (obtained from BART finetuned models on CNN dataset) correlates much strongly with the human factuality scores on the SummEval dataset (Table 4), as well as the summarization factuality datasets (i.e., Rank-19 and Q-CNN (Table 5)). 
Even though we think BARTScore metric can be a efficient to automatically evaluate faithfulness of the model generated output summaries on several domains, we present several hypothesis and arguments in the next that suggests that it may not generalize well for to the answer summarization model evaluations, hence we propose a new faithfulness evaluation score adapting the BARTScore. 

We start with the BARTScore formulation by \citet{yuan2021bartscore}, which is defined as  `` \emph{direct evaluation of text through the lens of its probability of being generated}''. Formally, the faithfulness of a \emph{generator model} $f$ is computed by another seq2seq \emph{verifier model} $v$ as $\bs[v]{g(X); X} = \log p_v(f(X) \mid X)$, where $p_v(\parg)$ is the probability assigned by $v$ to a sequence.
Thus, it is crucial that the verifier model $v$ used for computing the \bartscore{} be a good \emph{generative model} as well so that its generation probabilities ($p_v(\parg)$) have high \emph{statistical power}. We claim that using the vanilla \bartscore{} won't be efficient for the answer summarization model evaluation since vanilla \bartscore{} is trained on news articles (i.e., CNN/DM datasets) while our models are trained and evaluated on the post about users answers to open domain questions (i.e., CQA data), which has a different discourse structure and semantic features compared to news datasets.  
% This is because cannot be used for our purpose due to the domain shift between news articles and CQA data. 
As suggested in \citet{yuan2021bartscore}, this domain shift issue can be mitigated by fine-tuning the underlying BART model on the task data which would then yield an enhanced \bartscore{} for the task at hand.  We should also note that the human annotators generate the reference summaries of multiple answers given a question by using only the relevant sentences from the answers. How can we build a verifier model that not only adapts the features of \bartscore{} but also evaluates the faithfulness of the multi-answer summarization task simulating human's evaluation criteria?

\paragraph{Technical justification for using the Oracle model to measure faithfulness.}
In this section we give technical justification for using the Oracle model to measure faithfulness of all models. Since the Oracle model is trained on golden relevant sentences, using it to measure faithfulness of the standard BART (or T5) model against full answers might raise concerns around distribution shift. However, this distribution shift does not impact faithfulness scores meaningfully. Let us demonstrate our claim with an example: 
% To ground this in empirical demonstrations we performed the following experiment.
Denote the \bartscore{} computed using the Oracle BART model as $\bs[\mathrm{OBART}]{\parg}$, and the \bartscore{} computed using the standard BART model as $\bs[\mathrm{BART}]{\parg}$. On the test set we find:
\begin{align*}
    \bs[\mathrm{OBART}]{\mathrm{BART-rel}(Q, X); Q, X} &= -89.5 \\
    \approx \bs[\mathrm{OBART}]{\mathrm{OBART}(Q, R); Q, R} &= -87.1
\end{align*}
The BART-rel model is trained on relevant sentences but uses full answers at inference time (\S\ref{sec:baselines}).
%$\mathrm{OBART}(X)$ is the summary generated by the Oralce BART model when given the full answers $X$ as input --- we denote this model as BART-rel in Table \ref{tab:main_results} which is not an Oracle setting \asli{hmm, this is a tad confusing}. 
These results show that the Oracle BART model can be used to evaluate faithfulness with respect to full answers (long input). On the other hand, using the standard BART model as the verifier model produced very low faithfulness scores for the Oracle model:
\begin{align*}
 \bs[\mathrm{BART}]{\mathrm{OBART}(Q, R); Q, R} = -135.
\end{align*}
This justifies using the Oracle model to evaluate faithfulness of all models.

\paragraph{Faithfulness for extractive-abstractive models.}
There is one more problem with directly evaluating the faithfulness of an extractive-abstractive model $g$ as $\bs[\mathrm{OBART}]{g(X); X}$.
An ideal faithfulness metric assigns a probability $p_v(Y | X)$ to the output sequence $Y$ measuring the degree of faithfulness of $Y$ to $X$. For the purpose of evaluating the faithfulness of abstractive summaries, we will assume that sentence level extractive summaries are faithful, i.e., $p_v(Y | X) = 1$ if $Y$ is a sentence in $X$ \footnote{This may not be strictly true since it is possible to extract a single sentence from a paragraph that contradicts the information in the rest of the paragraph, e.g., sentences that express sarcasm. But such effects are minor in comparison to hallucinations in text generated by pre-trained language models.}. 
For extractive-abstractive models, the ideal faithfulness score factorizes as follows:
\begin{align}
    &\log p_v(Y \mid Q, X) \notag \\
    &\;= \sum_{i=1}^n \log p_v(R_i \mid Q, X_i) + \log p_v(Y \mid Q, R) \notag \\
    &\;= \log p_v(Y \mid Q, R). \label{eq:bart_score}
\end{align}
But $p_{\mathrm{OBART}}(R_i \mid Q, X_i) \gg 0$ and directly evaluating faithfulness of generated summary with respect to the full answers includes the effect of relevance sentence selection into the score --- there are better and more direct ways to evaluate the quality of relevant sentences (Table \ref{tab:rel_sent_pred}).
